# Supplementary material for: Differentiable Causal Backdoor Discovery
Source: arXiv:2003.01461 source file (2020-03-03)
Supplement: Supplementary file 1 [file appendix.tex]

The structural equations for the simulation benchmark are as follows:
% The structural equations for the continuous and discrete settings are as follows:
%U is an unobserved con-founder, and the rest of the variables are as described above. The random variables presented in the graph are distributed as follows.
\begin{equation}
\begin{aligned}[c]
        U \sim&\; \mathcal{N}(0,\mathbf{I}), \\
        U' \sim&\; \mathcal{N}(0,\mathbf{I}), \\
        W \sim&\; \mathcal{N}(0,1), \\
        \mathcal{Z}_1 \sim&\; \alpha_{\mathcal{Z}_1} W + \beta_{\mathcal{Z}_1} U + \gamma_{\mathcal{Z}_1} U' + \mathcal{N}(0, \sigma_{\mathcal{Z}_1}^2\mathbf{I}), \\
        \mathcal{Z}_2 \sim&\; \alpha_{\mathcal{Z}_2} W + \mathcal{N}(0,\mathbf{I}), \\
        \mathcal{Z}_3 \sim&\; \mathcal{N}(0, \sigma_{\mathcal{Z}_3}^2\mathbf{I}), \\
        \mathcal{Z}_4 \sim&\; \mathcal{N}(0,\mathbf{I}), \\
        X \sim&\; \alpha_X U + \boldsymbol{\theta}_{X,2}^\top \mathcal{Z}_2 + \boldsymbol{\theta}_{X,3}^\top \mathcal{Z}_3 + \mathcal{N}(0, \sigma_X^2) \\
        Y \sim&\; \beta_{Y} U' + \boldsymbol{\theta}_{Y,2}^\top \mathcal{Z}_2 + \boldsymbol{\theta}_{Y,4}^\top \mathcal{Z}_4 + \omega X + \mathcal{N}(0, \sigma_{Y}^2)
\end{aligned}
\end{equation}

\begin{algorithm*}[t!]
\caption{\textsc{DiscreteDiscovery}: Discover backdoor for discrete model.}\label{algo:discrete}
    {\bf Input:} \\
    Train Data: $\{w_i, y_i, x_i, \bb{z}_i\}_{i=1}^n = \bb{w}, \bb{y}, \bb{x}, \bb{Z}$ \\
    Validation Data: $\{\hat{w}_i, \hat{y}_i, \hat{x}_i, \hat{\bb{z}}_i\}_{i=1}^n = \hat{\bb{w}}, \hat{\bb{y}}, \hat{\bb{x}}, \hat{\bb{Z}}$ \\
    Parameters: $\theta \in \mathbb{R}^p$ \\
    Set of hyperparameters: $\Lambda, \alpha=10^{-8}$ \\
    {\bf Output:} \\
    ATE estimate: $\tau$ 
\begin{algorithmic}[1]
  \State $D = []$ \Comment{store validation results}
  \State $B = []$
  \For{$\lambda \in \Lambda$}
    \While{true} \Comment{make sure $W \nindep Y~|~ \beta^\top Z$}
    \State Initialize $\theta$
    \For{$t = 1, \ldots, T$} \Comment{Main learning loop}
      \State $\beta = \frac{\theta}{\|   \theta \|_2}$ 
      \State $\ell, \bb{g} =   \Call{ForwardBackward}{\bb{w},   \bb{y}, \bb{x}, \bb{Z}, \beta}$
      \State $\theta = \Call{ADAM}{\theta,   \bb{g}}$ \Comment{May need to project weights for sparsity}
    \EndFor
    \State $\beta = \frac{\theta}{\| \theta   \|_2}$ 
    \State Check if $\alpha$ is large enough:
    %\State $\bb{p}_w^x =   \Call{LogisticRegression}{\bb{w} = 1 |   \beta^\top \bb{Z}}$ \Comment{$p(W |   \beta^\top Z)$}
    %\State $\bb{p}_y^x =   \Call{LogisticRegression}{\bb{y} = 1 |   \bb{w}, \beta^\top \bb{Z}}$   \Comment{$p(Y | W, \beta^\top Z)$}
    %\State $d_x =   \Call{LogOdds}{\bb{p}_w^x, \bb{p}_y^x}$
    \State $d_{z} = \Call{LogOdds}{\bb{w}, \bb{y}, \{ \beta^\top \bb{Z}\}}$
    \If{$d_z$ passes significance test}
      \State break
    \EndIf
    \State $\alpha = 10^2 \alpha$
    \EndWhile
    % \State $\hat{\bb{p}}_w^{zx} =   \Call{LogisticRegression}{\hat{\bb{w}}   = 1 | \beta^\top \hat{\bb{Z}},   \hat{\bb{x}}}$ \Comment{$p(W |   \beta^\top Z, X)$}
    %   \State $\hat{\bb{p}}_y^{zx} =   \Call{LogisticRegression}{\hat{\bb{y}  } = 1 | \hat{\bb{w}}, \beta^\top   \hat{\bb{Z}}, \hat{\bb{x}}}$   \Comment{$p(Y | W, \beta^\top Z, X)$}
    %   \State $\hat{d}_{zx} =   \Call{LogOdds}{\hat{\bb{p}}_w^{zx},   \hat{\bb{p}}_y^{zx}}$ 
    \State $\hat{d}_{zx} = \Call{LogOdds}{\hat{\bb{w}}, \hat{\bb{y}}, \{ \beta^\top \hat{\bb{Z}}, \hat{\bb{x}}\}}$
      \State $D = [D, \hat{d}_{zx}]$
      \State $B = [B, \beta]$
  \EndFor
  \State $i^* = \argmin D$
  \State $\beta^* = B_{i^*}$
  \State \Return ATE =  $\Call{ComputeATE}{\beta^*, \bb{x}, \bb{Z}, \bb{y}}$
  \Statex
  
  \Function{ForwardBackward}{$\bb{w}, \bb{y}, \bb{x}, \bb{Z}, \beta, \lambda, \alpha$}
    %\State $\bb{p}_w^{zx} = \Call{LogisticRegression}{\bb{w} = 1 | \beta^\top \bb{Z}, \bb{x}}$ \Comment{$p(W | \beta^\top Z, X)$}
    %\State $\bb{p}_y^{zx} = \Call{LogisticRegression}{\bb{y} = 1 | \bb{w}, \beta^\top \bb{Z}, \bb{x}}$ \Comment{$p(Y | W, \beta^\top Z, X)$}
    \State $d_{zx} = \Call{LogOdds}{\bb{w}, \bb{y}, \{ \beta^\top \bb{Z}, \bb{x} \}}$ %\bb{p}_w^{zx}, \bb{p}_y^{zx}}$
    %\State $\bb{p}_w^x = \Call{LogisticRegression}{\bb{w} = 1 | \beta^\top \bb{Z}}$ \Comment{$p(W | \beta^\top Z)$}
    %\State $\bb{p}_y^x = \Call{LogisticRegression}{\bb{y} = 1 | \bb{w}, \beta^\top \bb{Z}}$ \Comment{$p(Y | W, \beta^\top Z)$}
    \State $d_z = \Call{LogOdds}{\bb{w}, \bb{y}, \{ \beta^\top \bb{Z} \}}$ %\bb{p}_w^x, \bb{p}_y^x}$
    \State $\ell = d_{zx} + \lambda \| \beta \|_1 + \alpha d_{z}$
    \State \Return $\ell, \frac{\partial \ell}{\theta}$
  \EndFunction
  \Statex
  
  \Function{LogOdds}{$\bb{w}, \bb{y}, \mathcal{C}$}%{$\bb{p}_w, \bb{p}_y$}
    \State $\bb{p}_w = \Call{LogisticRegression}{\bb{w} = 1 | \mathcal{C}}$ \Comment{$p(W | \mathcal{C})$}
    \State $\bb{p}_y = \Call{LogisticRegression}{\bb{y} = 1 | \bb{w}, \mathcal{C}}$ \Comment{$p(Y | W, \mathcal{C})$}
    \State $d = 0$
    \For{$i = 1, \ldots, n$}
        \State $p^i_{w0y0} = (1-p_y^i(w^i=0))(1 - p_w^i)$
        \State $p^i_{w1y0} = (1-p_y^i(w^i=1)) p_w^i$
        \State $p^i_{w0y1} = p_y^i(w^i=0)(1 - p_w^i)$
        \State $p^i_{w1y1} = p_y^i(w^i=1)p_w^i$
        \State $d = d + \log \Bigg( \frac{ p^i_{w0y0} p^i_{w1y1}    }{ p^i_{w0y1} p^i_{w1y0}} \Bigg)$
    \EndFor 
    \State \Return $d$
  \EndFunction
  \Statex
\algstore{myalg}
\end{algorithmic}
\end{algorithm*}
